# Supplementary material for: Joint Learning of Neural Networks via Iterative Reweighted Least Squares
Source: arXiv:1905.06526 source file (2019-06-11)
Supplement: Supplementary file 1 [file 07_appendix.tex]

\section{Objective Functions for the Homogeneous Case}

Suppose we have $m$ datasets. Each dataset consists of $n_i,1\leq i\leq m$ labeled feature pairs $\bs{x}_{ij}, y_{ij}, 1\leq j \leq n_i, 1\leq i \leq m$. We are interested in finding effectiveness solutions to the following two optimization problems:

\noindent\textbf{Formulation I.} We want to train $m$ support vector machines $(\bs{w}_i, b_i)$ to solve the following optimization problem:
\begin{align*}
\underset{(\bs{w}_i, b_i), 1\leq i \leq m}{\textup{minimize}} &\quad \Big( \sum\limits_{i=1}^{m}\big(\sum\limits_{j=1}^{n_i}\psi_{ij} + \lambda \|\bs{w}_i\|^2\big)\Big) \\
& + \mu \sum\limits_{1\leq i < i'\leq m}\|\bs{w}_i-\bs{w}_{i'}\|^2 \\
\textup{subject to} &\quad  y_{ij}\cdot (\bs{w}_i^{T}\bs{x}_{ij}+b_i) \geq 1- \psi_{ij}, \\
&\quad \psi_{ij}\geq 0, 
\begin{array}{c}
\quad 1\leq j \leq n_i \\
1\leq i \leq m
\end{array}
\end{align*}

\noindent\textbf{Formulation II.} The second formulation uses logistic regression:
\begin{align*}
\underset{(\bs{w}_i, b_i), 1\leq i \leq m}{\textup{minimize}} &\quad \Big( \sum\limits_{i=1}^{m}\big(\sum\limits_{j=1}^{n_i}(\frac{e^{\bs{w}_i^{T}\bs{x}_{ij}+b_i}}{e^{\bs{w}_i^{T}\bs{x}_{ij}+b_i}+1}-\frac{1+y_{ij}}{2})^2 \\
&\quad + \lambda \|\bs{w}_i\|^2\big)\Big) + \mu \sum\limits_{1\leq i < i'\leq m}\|\bs{w}_i-\bs{w}_{i'}\|_1 \\
\end{align*}

For optimization, we can augment the objective function so that it becomes
\begin{align*}
\underset{(\bs{w}_i, b_i), 1\leq i \leq m}{\textup{minimize}} &\quad \Big( \sum\limits_{i=1}^{m}\big(\sum\limits_{j=1}^{n_i}(\frac{e^{\bs{w}_i^{T}\bs{x}_{ij}+b_i}}{e^{\bs{w}_i^{T}\bs{x}_{ij}+b_i}+1}-\frac{1+y_{ij}}{2})^2 \\
&\quad + \lambda \|\bs{w}_i\|^2\big)\Big) + \mu \sum\limits_{1\leq i < i'\leq m}\|\bs{w}_i-\bs{w}_{i'}\|_1 \\
& \quad + \gamma \sum\limits_{1\leq i < i'\leq m}\|\bs{w}_i-\bs{w}_{i'}\|^2
\end{align*}
The objective function becomes smooth now, and we can apply alternating minimization for optimization.
